# Supplementary material for: QCD Physics Potential of CMS
Source: arXiv:0911.3072 source file (2009-11-16)
Supplement: Supplementary file 1 [file Appendix.tex]

% Authors: To whom it may concern
\section{Appendix}
